# Supplementary material for: Gemini NIFS survey of feeding and feedback processes in nearby Active Galaxies: VI -- Stellar Populations
Source: arXiv:2203.07484 source file (2022-03-18)
Supplement: Supplementary file 1 [file SupMat.pdf]

# Supplementary Material for Gemini NIFS survey of feeding and feedback processes in nearby Active Galaxies: VI - Stellar Populations

Maps and profiles for individual sources.

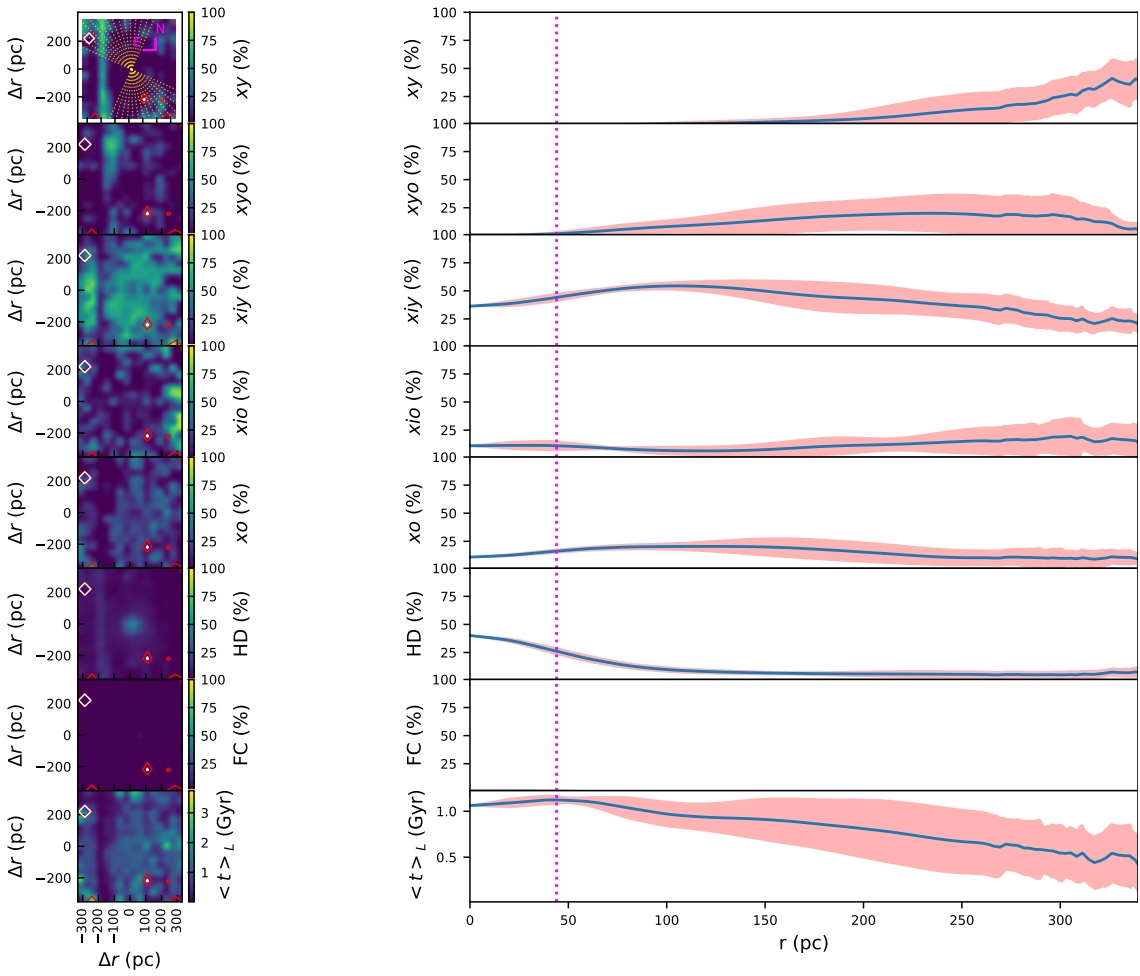

**Figure 1.** The same as Fig. 3 but for NGC 788

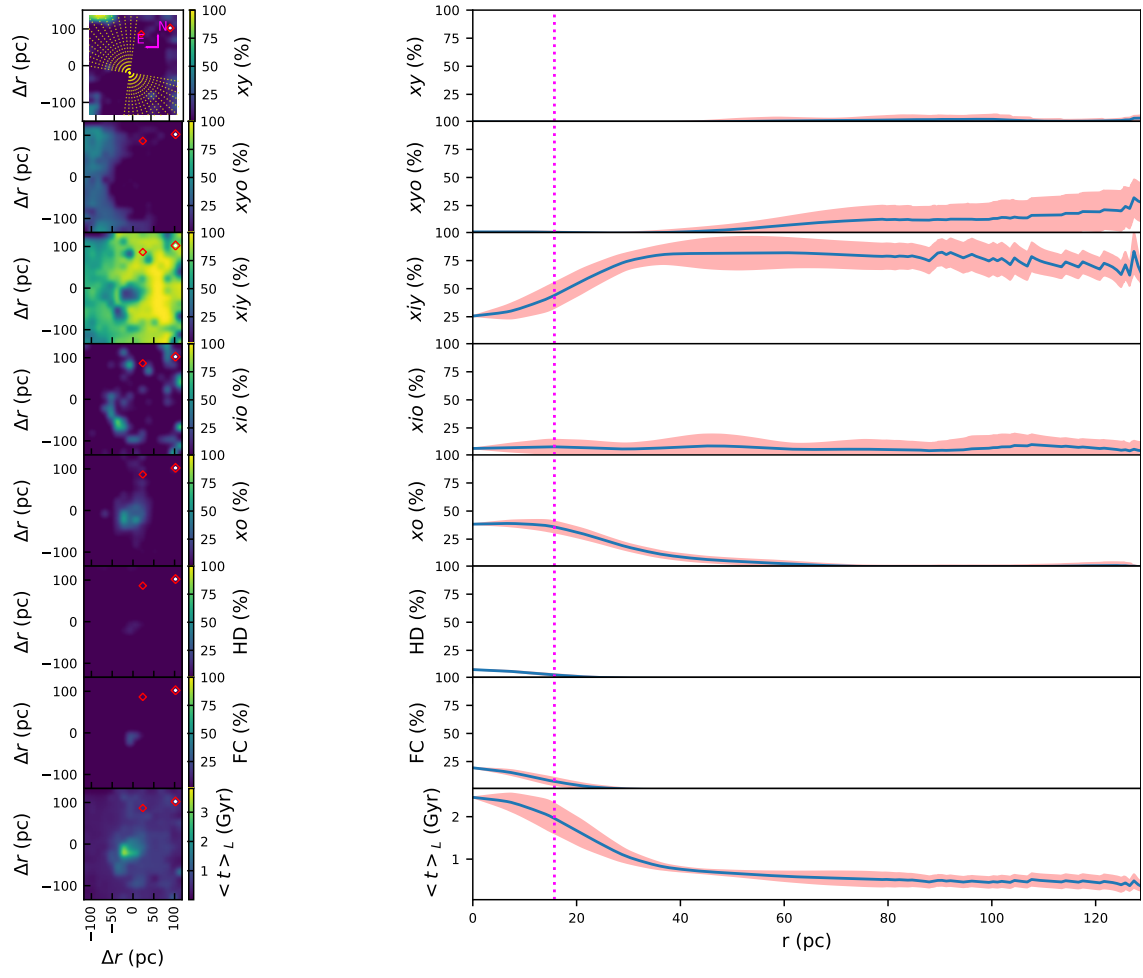

**Figure 2.** The same as Fig. 3 but for NGC 1052. The results of the stellar population synthesis are discussed [Dahmer-Hahn et al. \(2019\)](#).

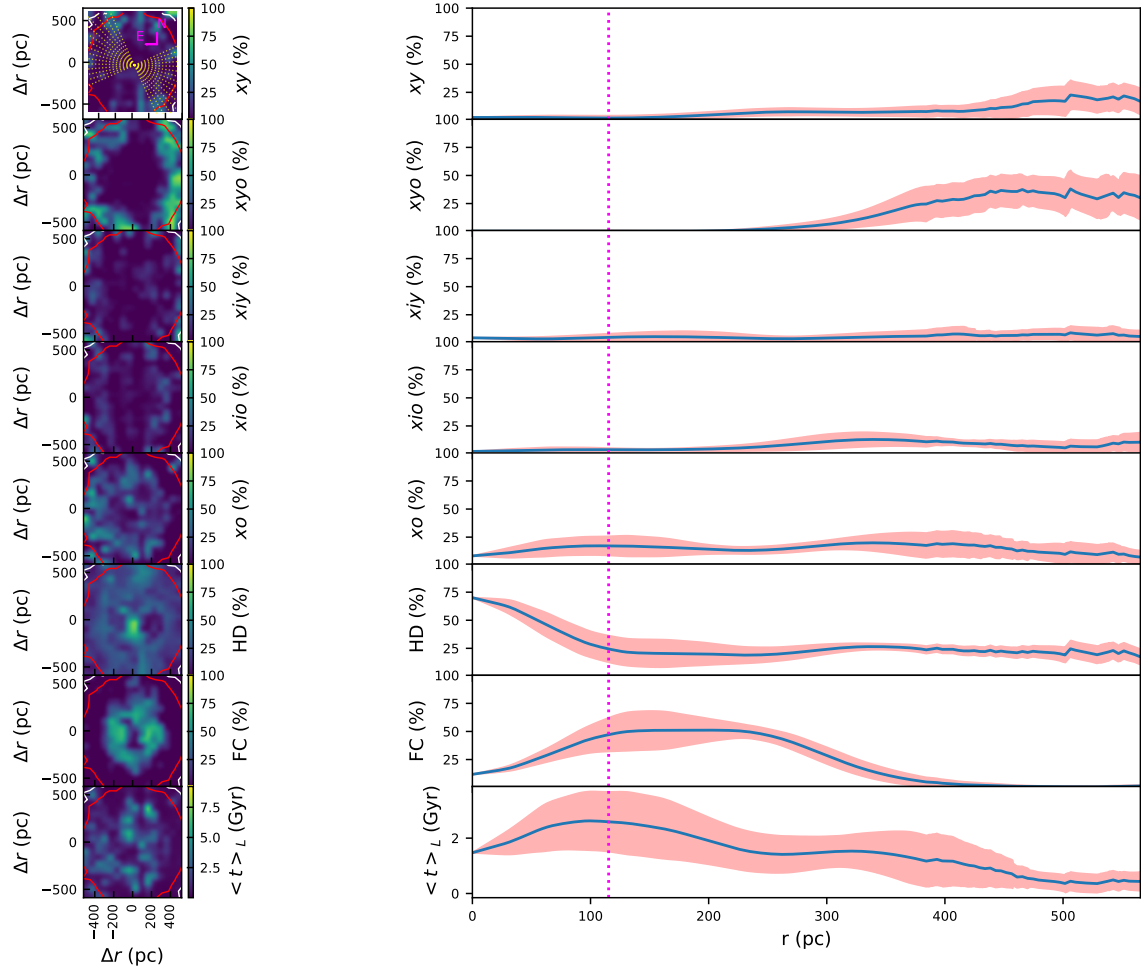

**Figure 3.** The same as Fig. 3 but for Mrk 79

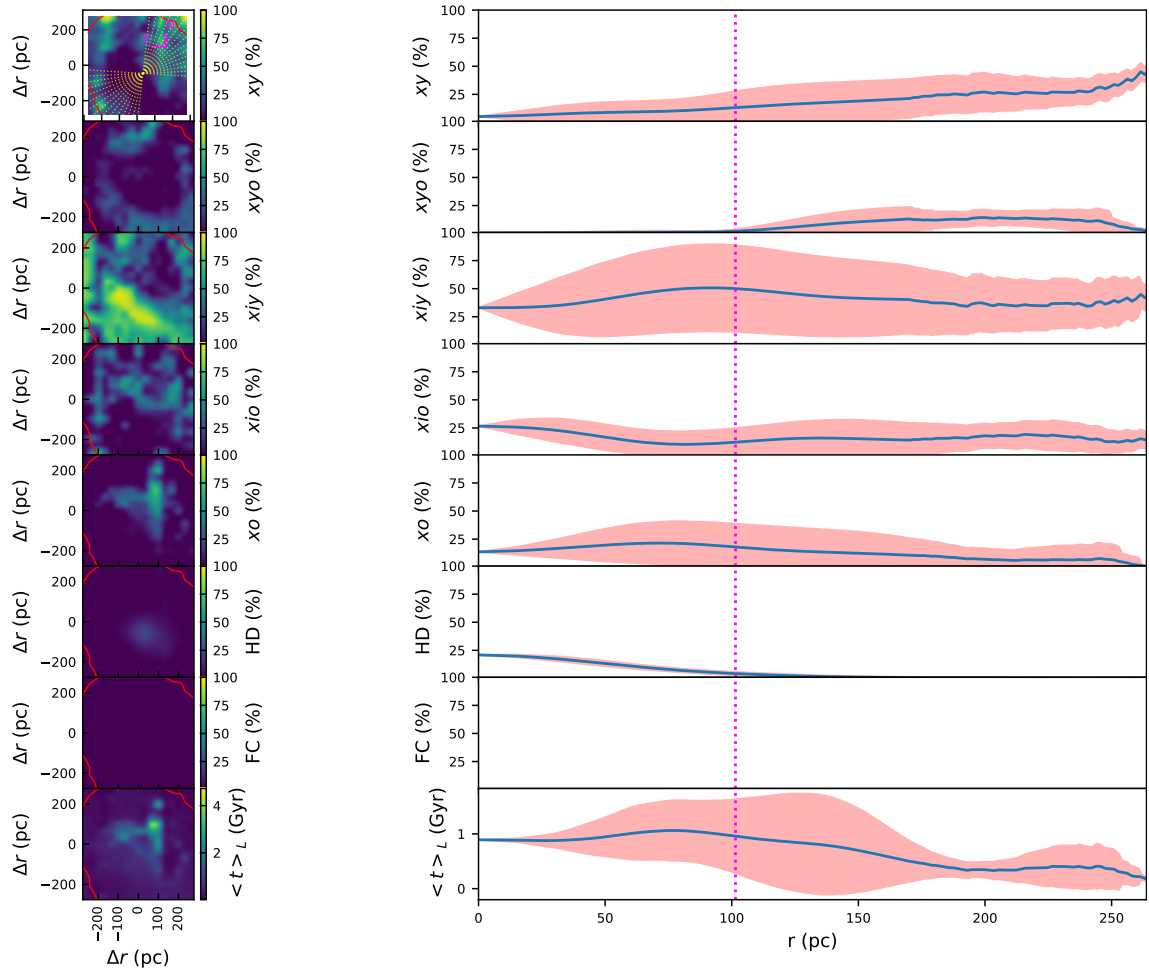

**Figure 4.** The same as Fig. 3 but for NGC 1125

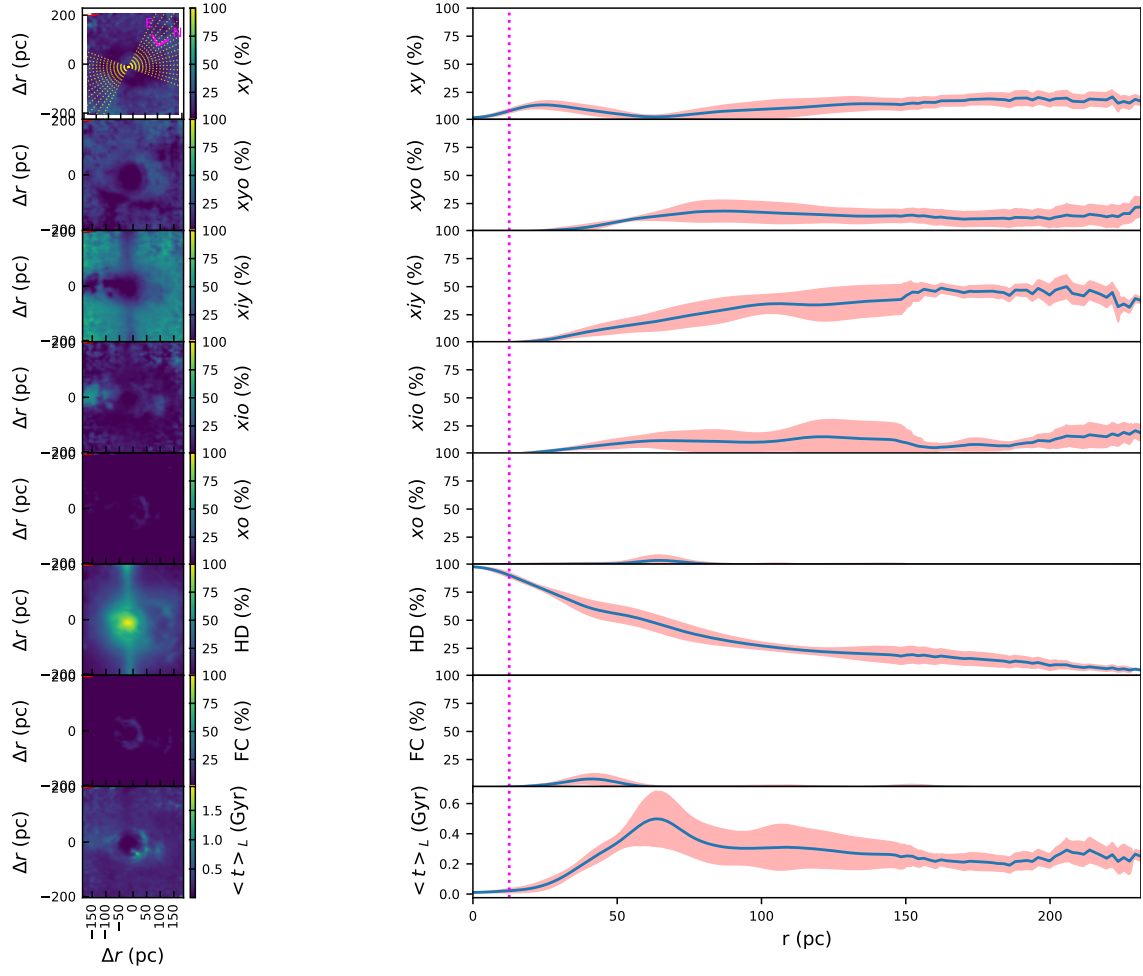

**Figure 5.** The same as Fig. 3 but for NGC1068. The results of the stellar population synthesis are discussed in [Storchi-Bergmann et al. \(2012\)](#)

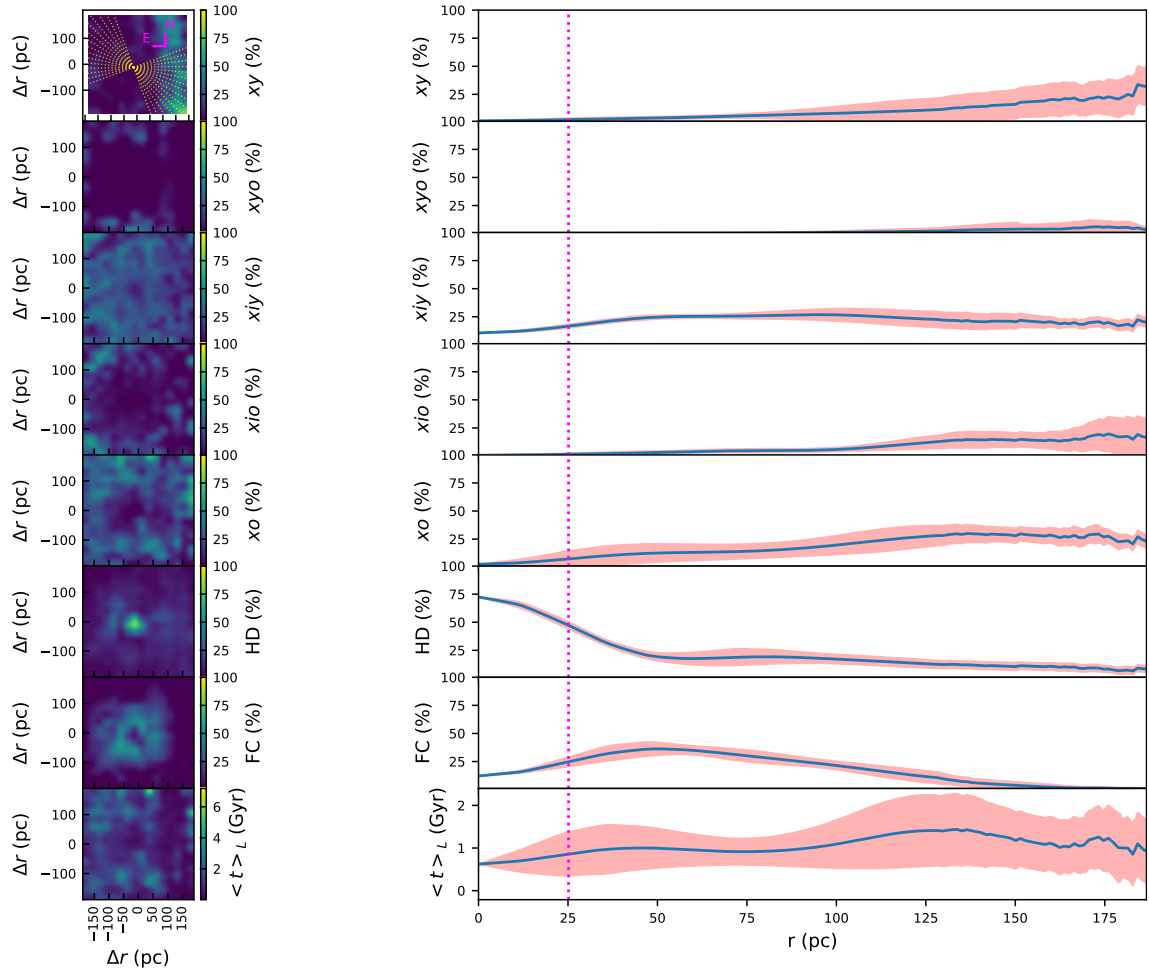

**Figure 6.** The same as Fig. 3 but for NGC2110. The results of the stellar population synthesis are discussed in [Diniz et al. \(2019\)](#).

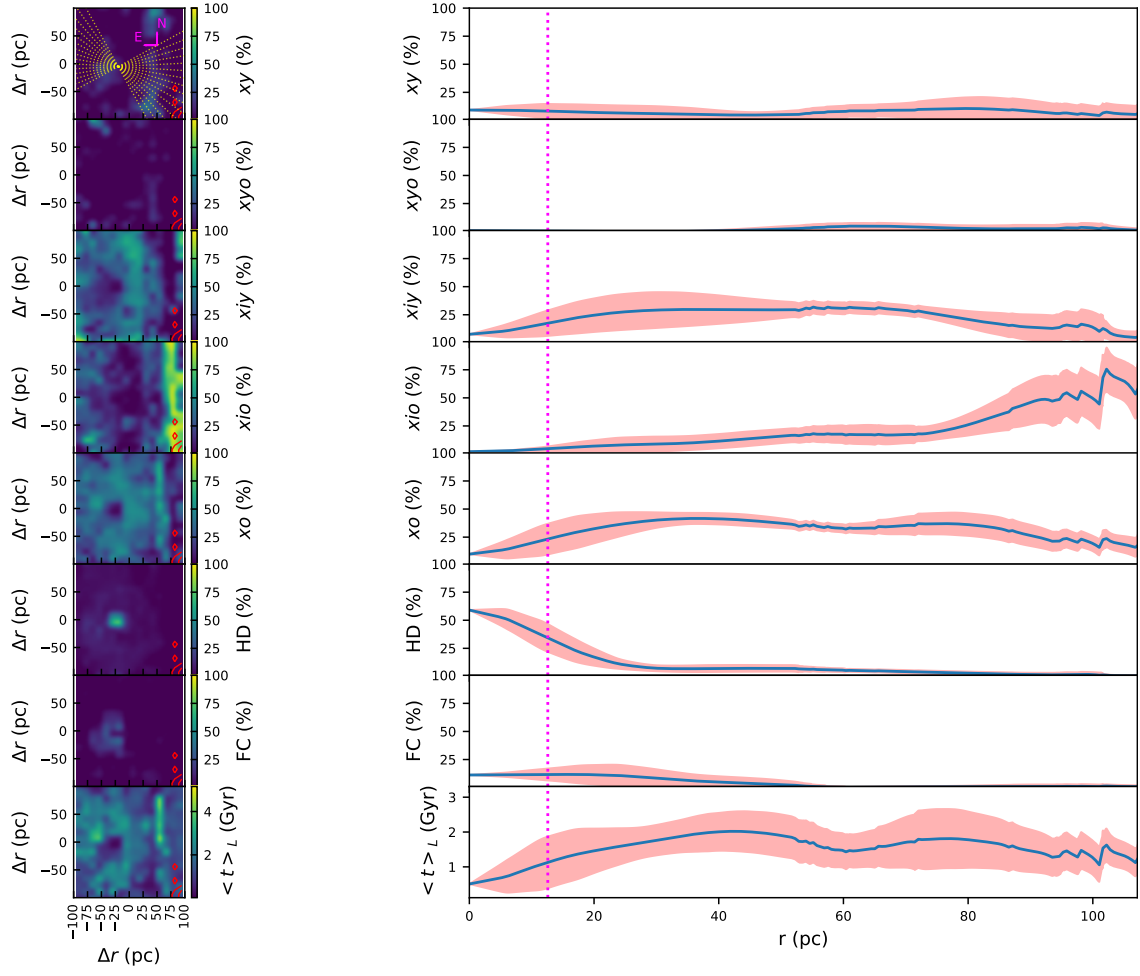

**Figure 7.** The same as Fig. 3 but for NGC 3227

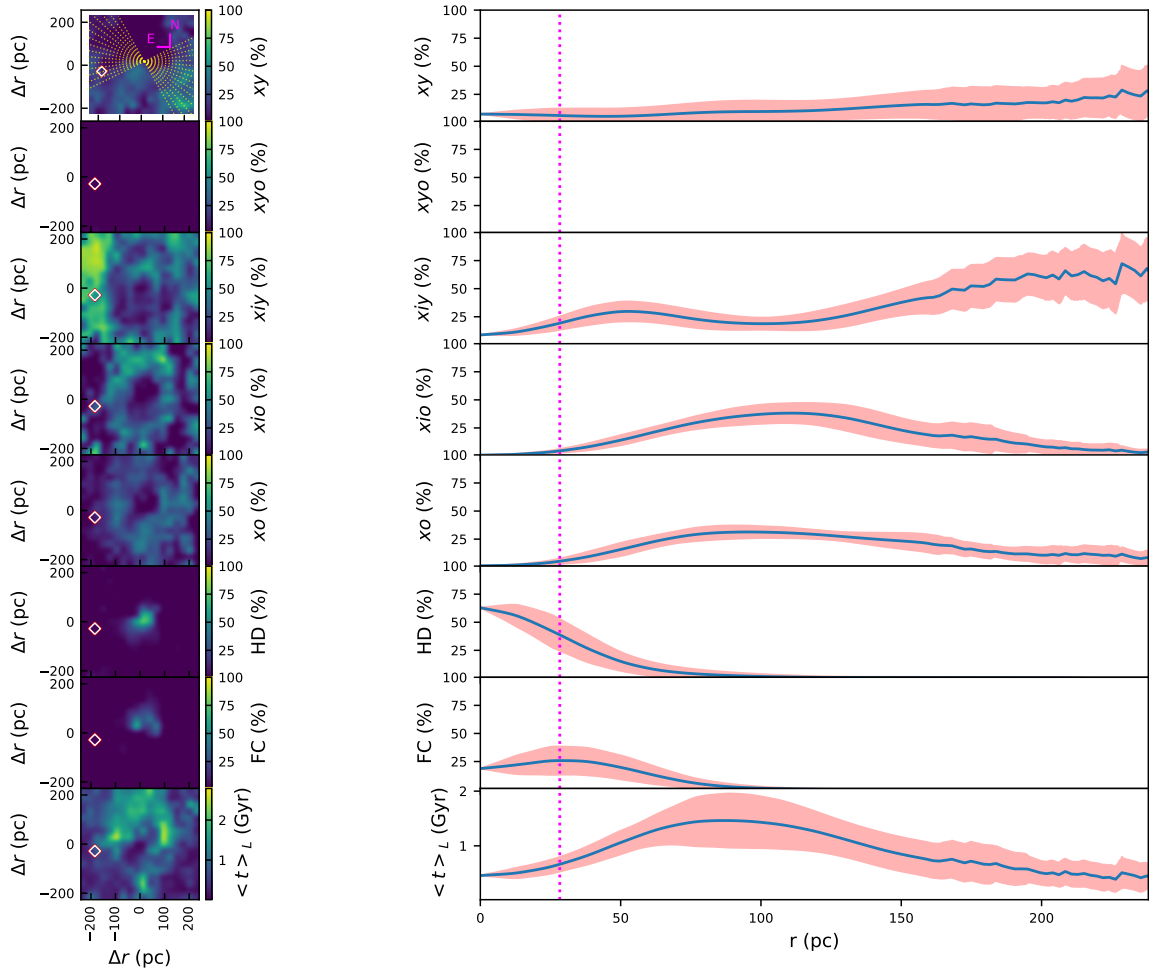

**Figure 8.** The same as Fig. 3 but for NGC 3516

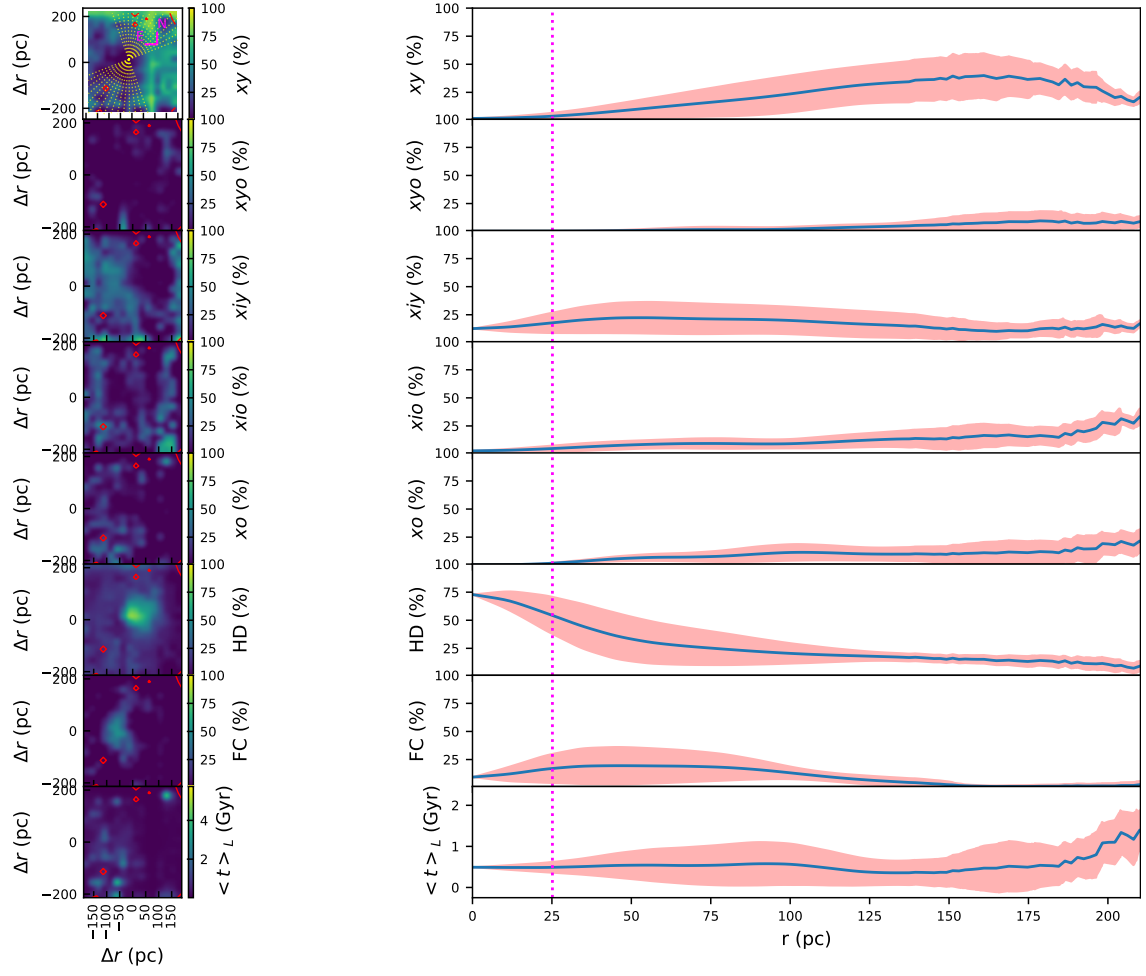

**Figure 9.** The same as Fig. 3 but for NGC4235

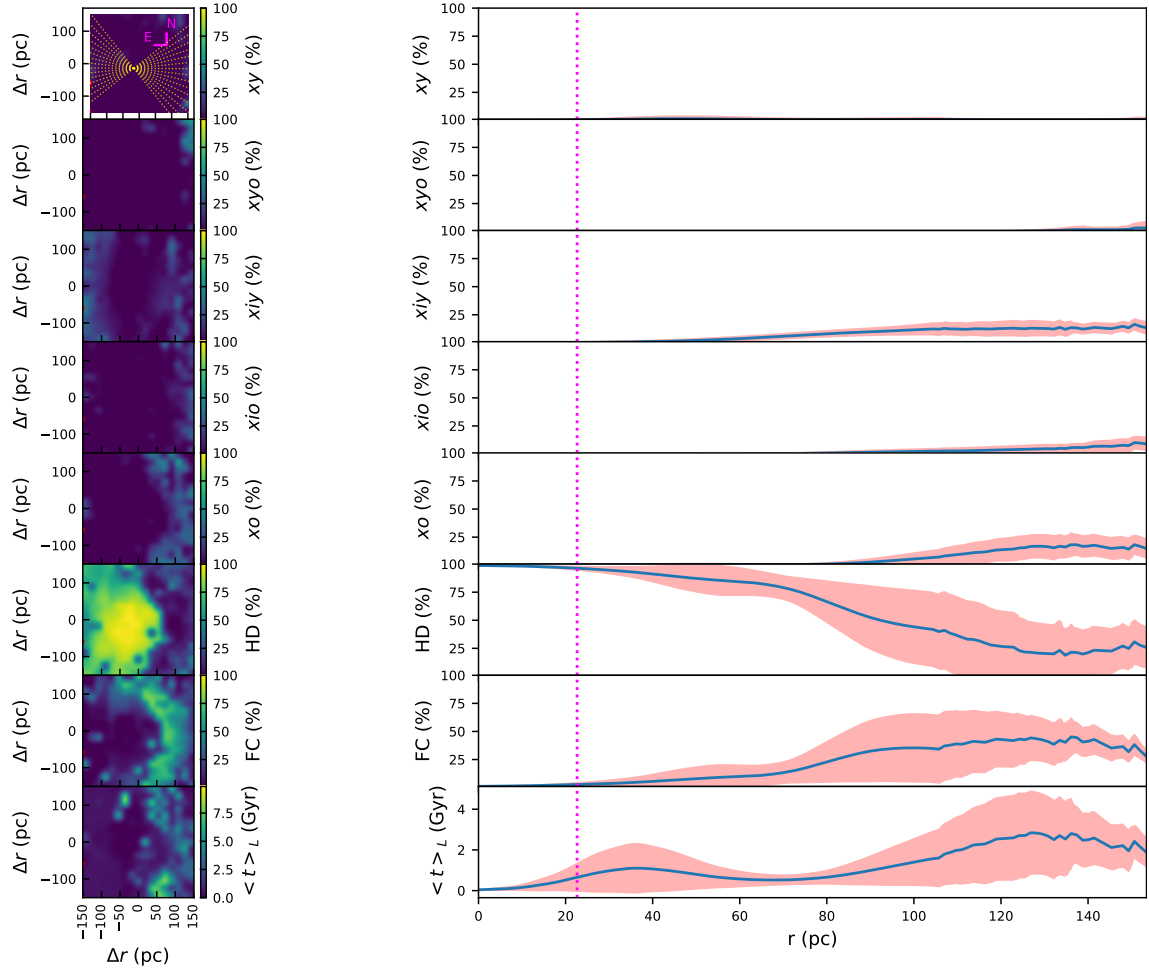

**Figure 10.** The same as Fig. 3 but for NGC5506

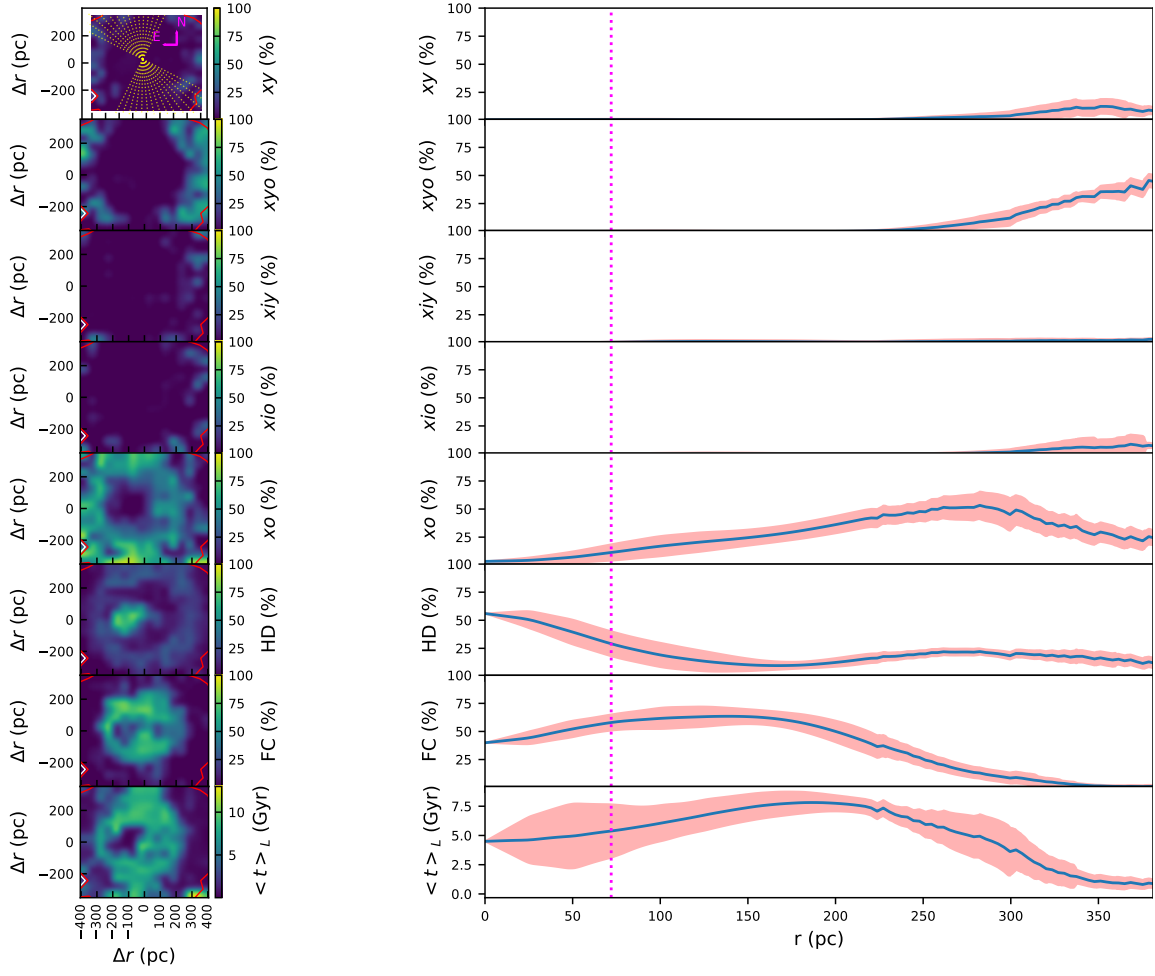

**Figure 11.** The same as Fig. 3 but for NGC5548. The results of the stellar population synthesis are discussed in (Schönell et al. 2017)

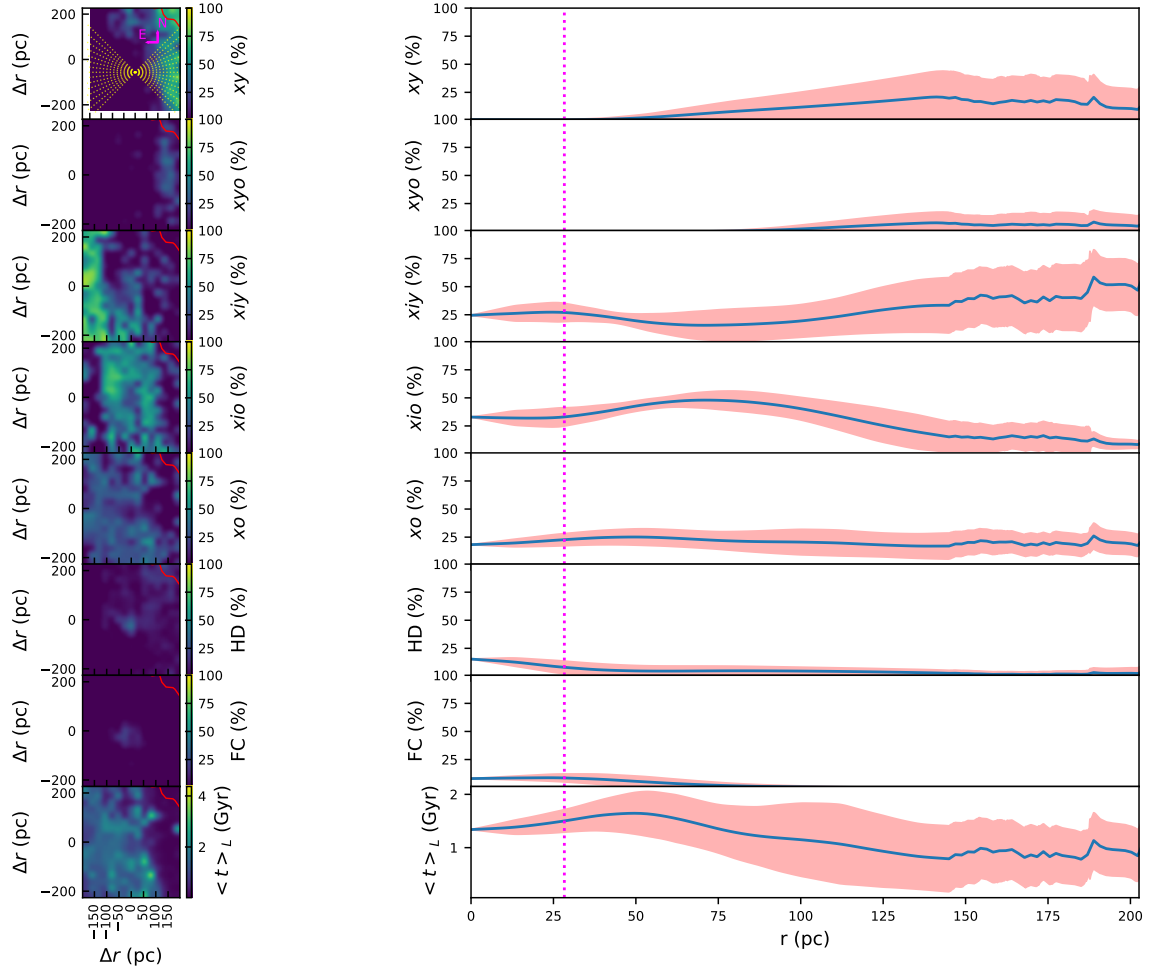

**Figure 12.** The same as Fig. 3 but for NGC5899

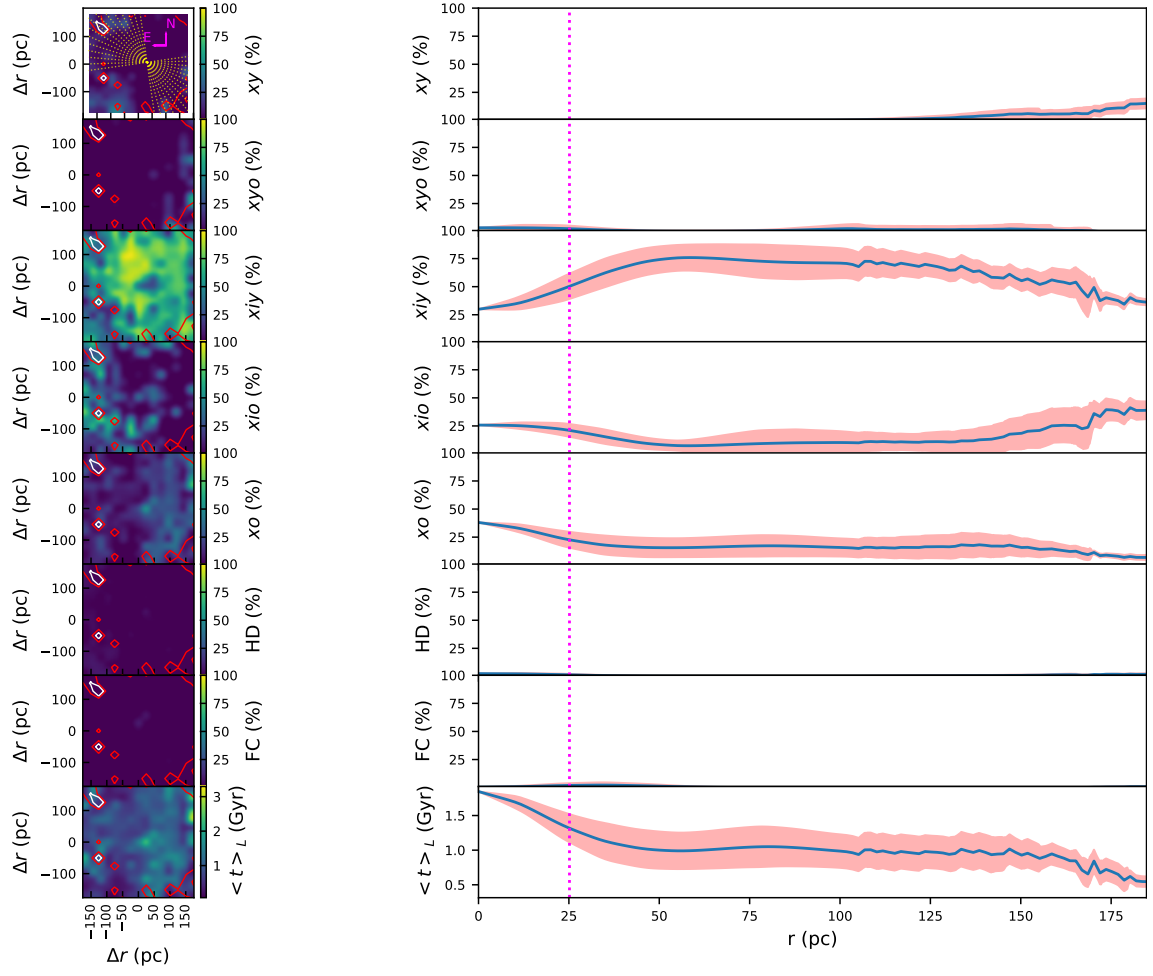

**Figure 13.** The same as Fig. 3 but for NGC5929

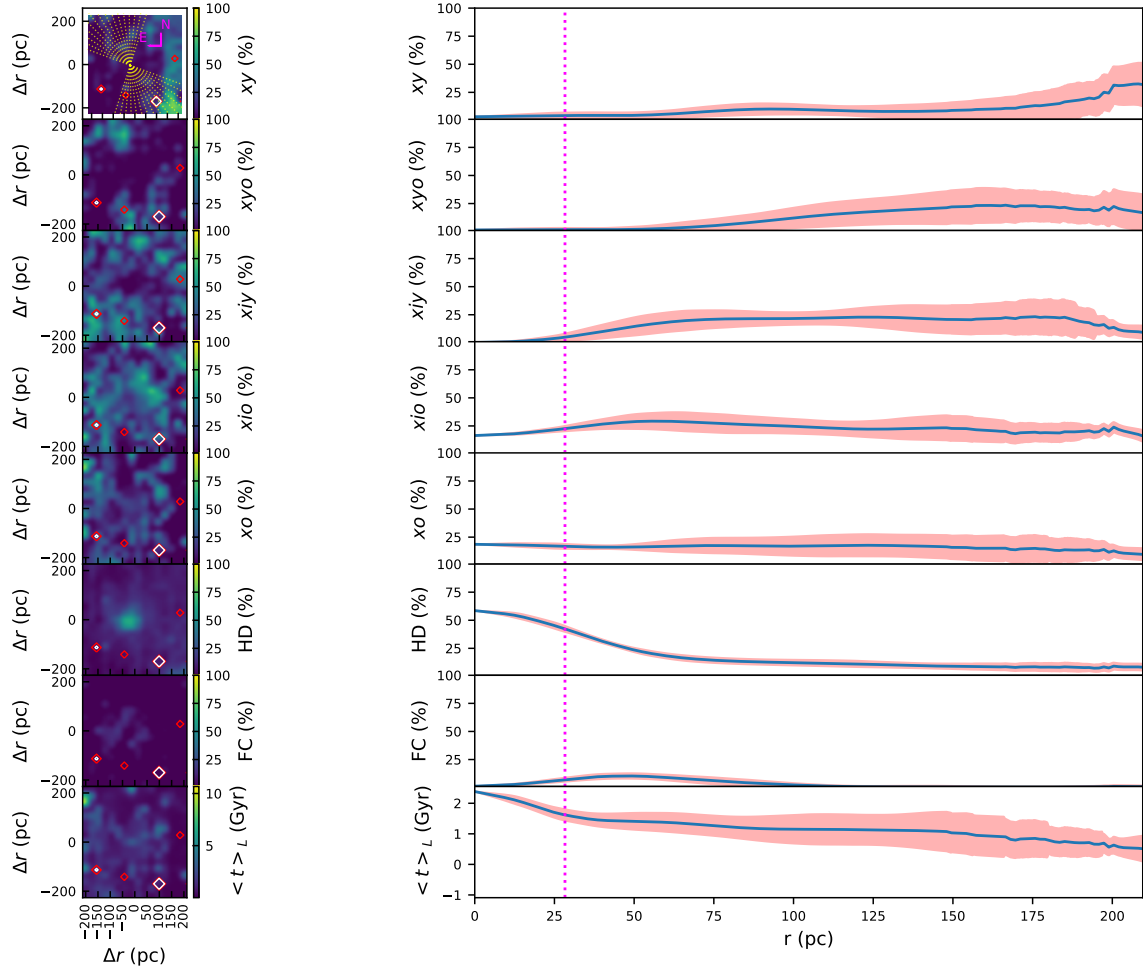

**Figure 14.** The same as Fig. 3 but for Mrk607

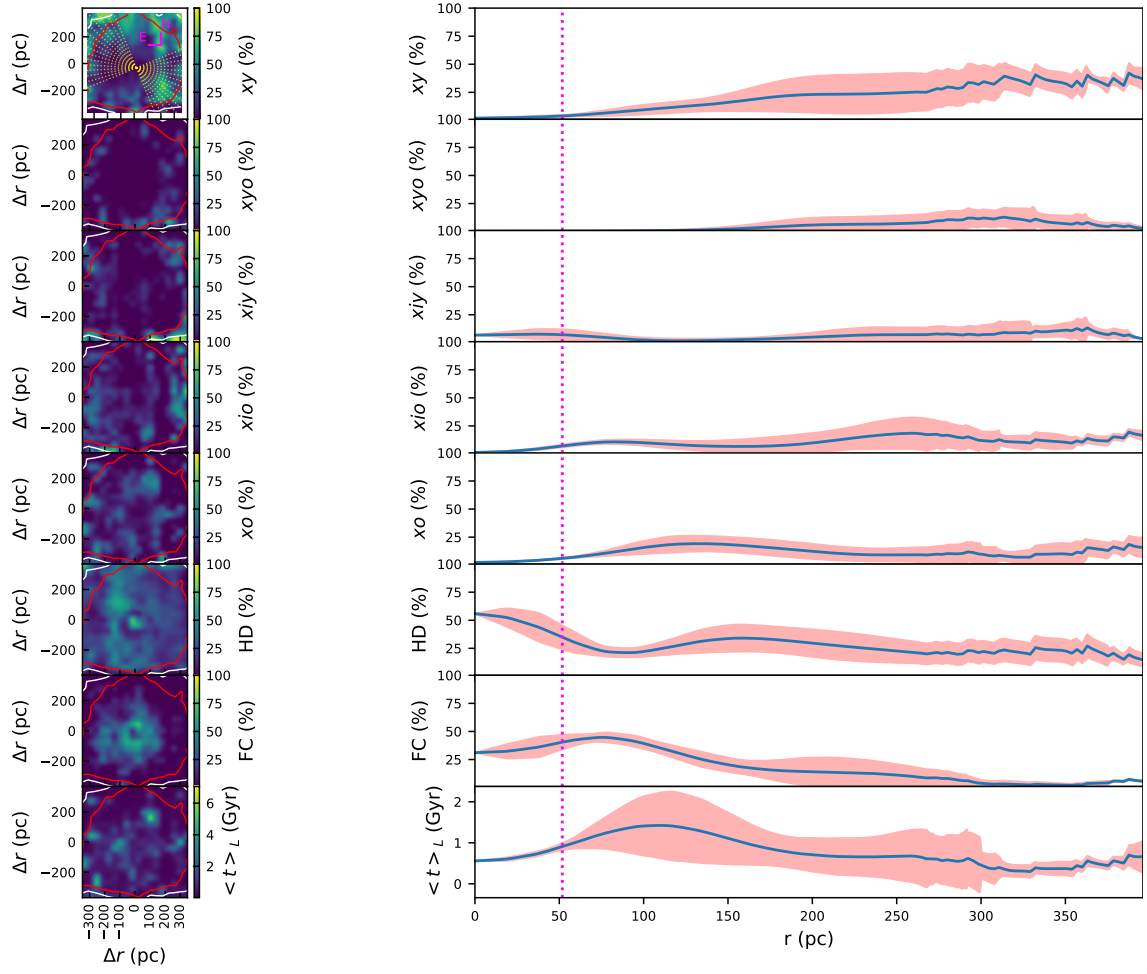

**Figure 15.** The same as Fig. 3 but for Mrk766

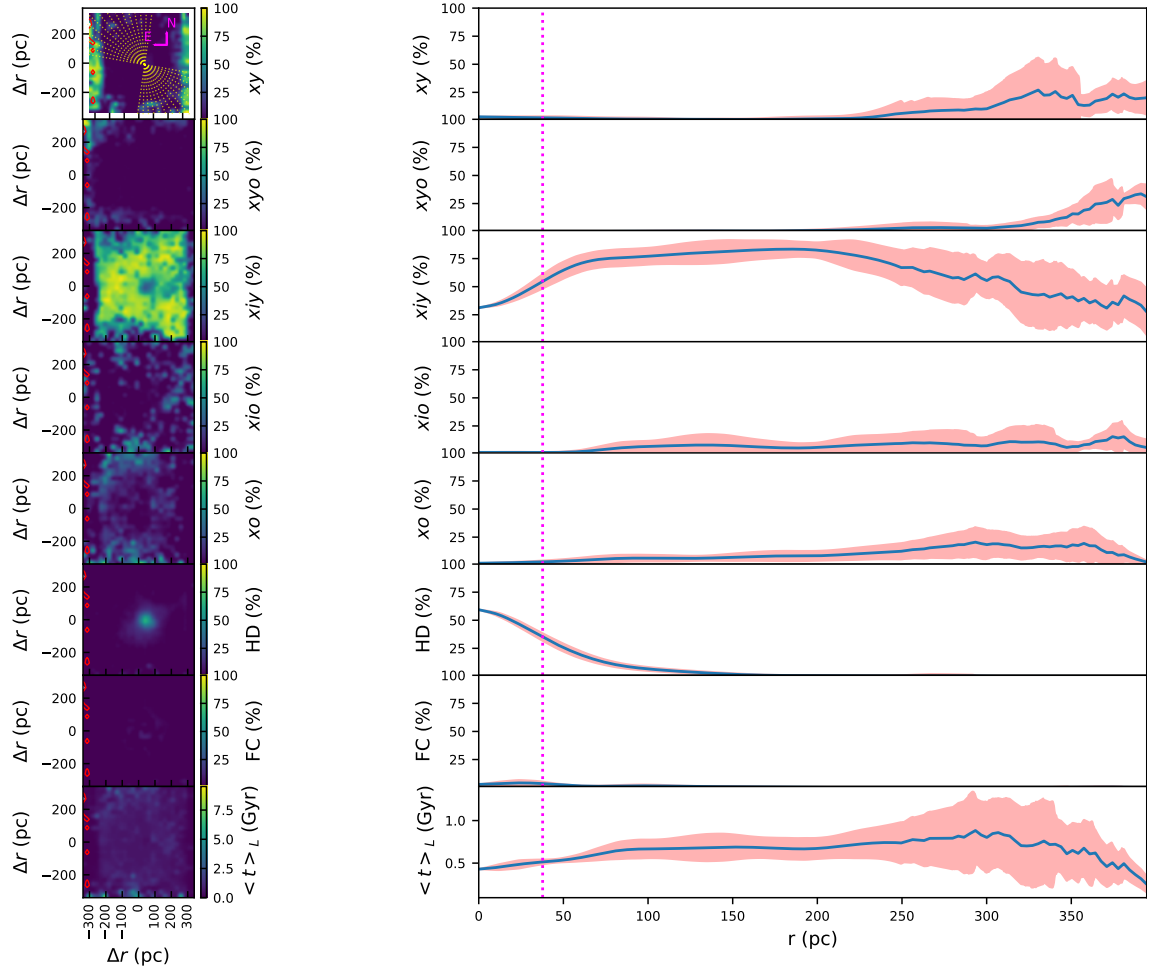

**Figure 16.** The same as Fig. 3 but for Mrk 1066. The results of the stellar population synthesis are discussed in [Riffel et al. \(2010\)](#).

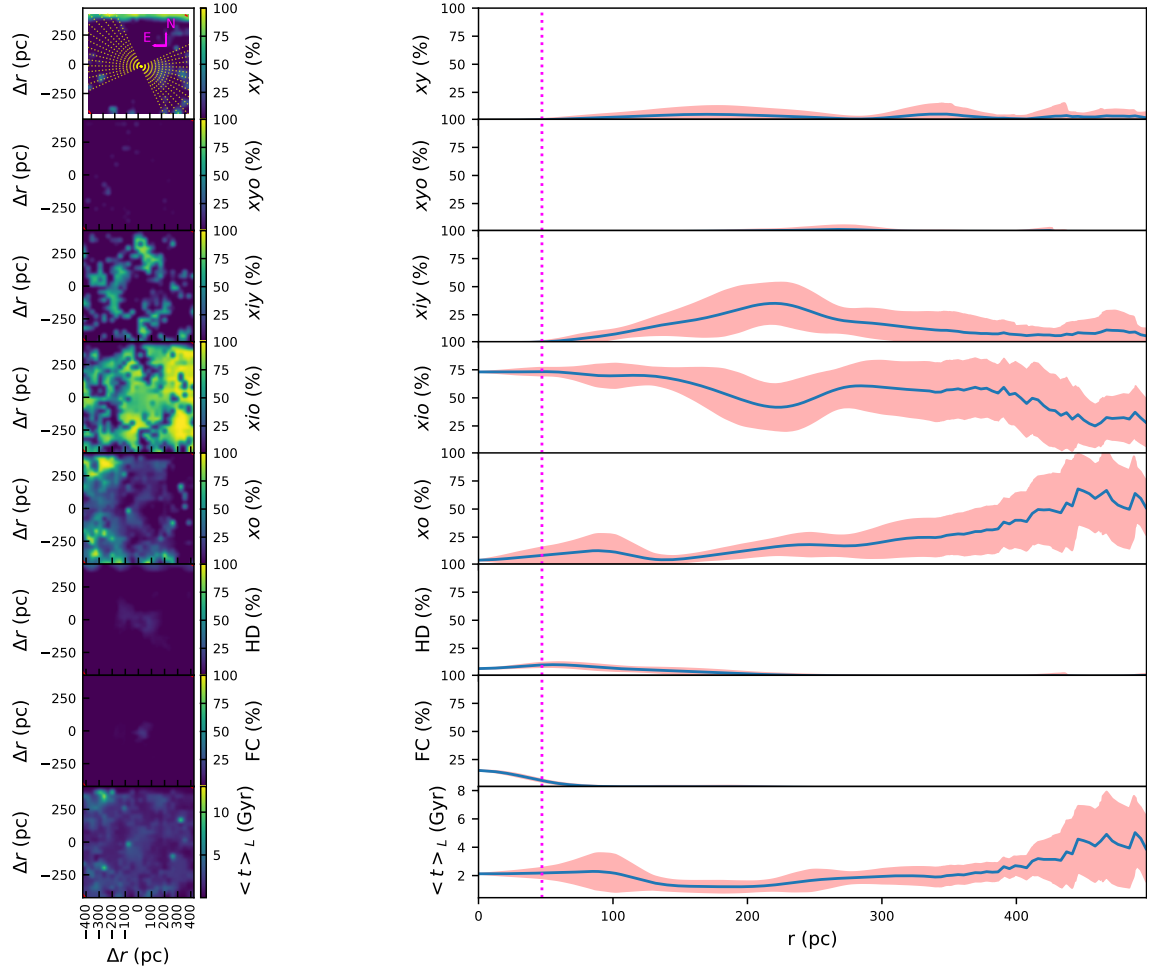

**Figure 17.** The same as Fig. 3 but for Mrk 1157. The results of the stellar population synthesis are discussed in [Riffel et al. \(2011\)](#)

**REFERENCES**

- Dahmer-Hahn L. G., et al., 2019, [Monthly Notices of the RAS](#), 482, 5211
- Diniz M. R., Riffel R. A., Storchi-Bergmann T., Riffel R., 2019, [Monthly Notices of the Royal Astronomical Society](#), 487, 3958
- Riffel R. A., Storchi-Bergmann T., Riffel R., Pastoriza M. G., 2010, [Astrophysical Journal](#), 713, 469
- Riffel R., Riffel R. A., Ferrari F., Storchi-Bergmann T., 2011, [Monthly Notices of the RAS](#), 416, 493
- Schönell Jr. A. J., Storchi-Bergmann T., Riffel R. A., Riffel R., 2017, [Monthly Notices of the Royal Astronomical Society](#), 464, 1771
- Storchi-Bergmann T., Riffel R. A., Riffel R., Diniz M. R., Borges Vale T., McGregor P. J., 2012, [Astrophysical Journal](#), 755, 87

This paper has been typeset from a  $\text{\TeX}/\text{\LaTeX}$  file prepared by the author.
